# Supplementary material for: Learning from Imperfect Human Feedback: a Tale from Corruption-Robust Dueling
Source: arXiv:2405.11204 source file (2024-10-14)
Supplement: Supplementary file 1 [file appendix-A.tex]

\counterwithin{lemma}{section}
\counterwithin{assumption}{section}
\counterwithin{definition}{section}
\counterwithin{proposition}{section}
\counterwithin{algocf}{section}
\counterwithin{figure}{section}
\section{Connection between Imperfect User and Generalized Learnability} \label{sec:appendix_A}
In this section, we establish the connection between adversarial corruption, corruption induced by generalized learnability, and corruption induced by $\rho$-\emph{imperfect} user. Broadly speaking, holding total corruption budget $C$ constant, corruption induced by generalized learnability is a specific type of \emph{arbitrary} corruption. Furthermore, if the proposed action pairs exhibit sufficient diversity, corruption induced by $\rho$-\emph{imperfect} user is equivalent to corruption induced by generalized learnability. 

In the following, we introduce the concept of the generalized learnability of the utility function $\mu$ in the scenario of pairwise comparison and the associated corruption induced throughout the user's learning process.

\begin{definition}[Corruption induced by Generalized Learnability]\label{def:generalized_learnability}
    There exists an algorithm $\cG$ such that, given any arbitrary $t$ pairs of actions $\{a_s, a'_s\}^t_{s=1}$ and the associated utility differences $\{y_s\}^t_{s=1}$, where $ y_s := \mu(a_s) - \mu_(a'_s)$, $\cG$ can output an estimated utility function $\mu_t : \bR^d \rightarrow \bR$ of the true utility function $\mu: \bR^d \rightarrow \bR$ such that for any action pair $(a, a')$ the following equation holds 
    \begin{align*}
            |c_t(a, a')| = |\mu_t(a) - \mu(a) - (\mu_t(a') - \mu(a'))| \leq C_0 \left(\|a-a'\|^2_{\bar V_t^{-1}}\right)^{1 - \rho}.
    \end{align*}
    $C_0$ is some positive constant, $\rho \in [0, 1]$, and $\bar V_t := \lambda \bI_d + \sum^t_{s = 1}(a_s - a'_s)(a_s - a'_s)^{\top}$, where $\lambda$ is some positive constant to ensure that $\bar V_t$ is full rank.
\end{definition}
Def. \ref{def:generalized_learnability} is a variant of the generalized learnability assumption proposed by \cite{wang2023followups} and \cite{yao2022learning}. Essentially, the parameter $\rho$ can be viewed as the user's irrationality level. A higher value of $\rho$ implies lower learning speed of the user's utility function $\mu$, hence a larger magnitude of the total induced corruption. Let's consider \emph{arbitrary} corruption with total corruption budget $C = \Theta(T^{\rho})$. Using Lemma \ref{lemma:A1}, we can show that $c_t(a, a')$ induced by the generalized learnability of $\mu$ satisfies $\sum^{T}_{t=1}|c_t(a_t, a'_t)| \leq O(T^{\rho})$, implies that it is a specific type of \emph{arbitrary} corruption.

In the scenario when $\lambda_{\min}(\bar V_t)$ increases in the order of $\Theta(t)$, $(\|a-a'\|^2_{\bar V^{-1}_t})^{1-\rho}$ has the order $\Theta(t^{\rho-1})$, which implies there exists a positive constant $C_{\kappa}$ that at round $t$, given arbitrarily proposed action pairs $(a, a')$, the magnitude of corruption $|c_t(a, a')| \leq C_{\kappa}t^{\rho -1}$, which means that corruption induced by a $\rho$-\emph{imperfect} user coincides with corruption induced by the generalized learnability of $\mu$.

We would like to highlight that the condition which $\lambda_{\min}(\bar V_t)$ increases in the order of $\Theta(t)$ could be satisfied by gradient-descent based algorithm. Take Algorithm \ref{algo:DBGD} as an example. For simplicity, let's assume $a^*$ is far away from the boundary of $\cA$ and projection never happens. It implies that $a'_t = a_t  + \delta u_t, \forall t \in [T]$. This assumption is without loss of generality, since most of the proposed action $a'_t$ will belong to the interior of the \emph{action} space $\cA$. This is because we start with $a_0 = 0$ and has small exploration size $\delta \sim \Theta(T^{-\alpha})$. Roughly speaking, we can express $\bar V_t = \lambda \mathbb{I}_d + \delta^2 \sum^t_{s=1}u_su^{\top}_s$, where $u_s$ is uniformly sampled from $\mathbb{S}^d$. Then applying Lemma \ref{lemma:A2}, we have $\lambda_{\min}(\bar V_t) \sim \Theta(t)$ with high probability.

\begin{lemma}[Generalized Elliptical Lemma in \cite{wang2023followups}]\label{lemma:A1}
Suppose $V_0 \in \bR^{d \times d}$ is any positive definite matrix, $a_1, \ldots, a_T \in \bR^{d}$ is a sequence of vectors with bounded $l_2$ norm and $\bar{V}_t  := V_0 + \sum^t_{s = 1}a_s a^{\top}_s$. Then for any $\rho \in [0, 1]$, the following inequality holds with probability at least $1 - \delta$
\begin{equation*}
    \sum^T_{t=1}\left(\min\left\{1, \|a_t\|^2_{\bar{V}^{-1}_t}\right\}\right)^{1-\rho} \leq 2^{1-\rho}T^{\rho}\log^{1-\rho}\left(\frac{\det(\bar{V}_t)}{\det(V_0)}\right).
\end{equation*}
\end{lemma}

\begin{lemma}[Proposition 1 in \cite{li2017provably}]\label{lemma:A2}
    Define $V_t := \sum^t_{s=1}u_s u^{\top}_s$, where $u_s$ is drawn iid from some distribution $\nu$ with support on the unit ball, $\mathbb{B}^d$. Furthermore, let $\Sigma:=\bE[u_su^{\top}_s]$ be the second moment matrix. $B$ and $\delta >0$ are two positive constants. Then, there exist positive, universal constants $C_1$ and $C_2$ such that $\lambda_{\min}(V_s) \geq B$ with probability at least $1 - \delta$, as long as 
    \begin{equation*}
        t \geq \left(\frac{C_1\sqrt{d} + C_2\sqrt{\log(1/\delta)}}{\lambda_{\min}(\Sigma)}\right)^2 + \frac{2B}{\lambda_{\min}(\Sigma)}.
    \end{equation*}
\end{lemma}
