# Supplementary material for: Learning from Imperfect Human Feedback: a Tale from Corruption-Robust Dueling
Source: arXiv:2405.11204 source file (2024-10-14)
Supplement: Supplementary file 2 [file appendix-D.tex]

\section{Additional Experiments}\label{sec:additional_experiments}
In this section, we list all the experiment details. At the beginning, we introduce the regret order fitting method, different types of corruption that we simulate in the experiments, and baseline algorithms for comparison.

\vspace{10pt}
\noindent  \textbf{Fitted Order of Regret.} We introduce the methodology that we use to compute the order of $\text{Reg}_T$ in terms of the number of iteration, $T$. To fit the order of the regret, we first convert it into $\log$ scale. Then we input the last $1\%$ of data, run linear regression, and use ordinary least squares to estimate the slope of the line, which is the \emph{fitted order} of $\text{Reg}_T$.

\vspace{10pt}
\noindent  \textbf{Corruption.} In the experiments, we consider two types of corruption: corruption induced by $\rho$-\emph{imperfect} user and \emph{arbitrary} corruption. For corruption induced by $\rho$-\emph{imperfect} user, we simulate $c_t(a_t, a'_t)$ according to Definition \ref{def:generalized_learnability}. We set $\lambda = 2$ and $C_0 = 0.1(\max_{a \in \cA} \mu(a) - \min_{a \in \cA}\mu(a))$. Moreover, we add $c_t(a_t, a'_t)$ to the utility difference of $a_t$ and $a'_t$ adversarially. In particular, if $\mu(a_t) > \mu(a'_t)$, then $\hat \bP(a_t \succ a'_t) = \sigma(\mu(a_t) - \mu(a'_t) - c_t(a_t, a'_t))$, then vice versa. For \emph{arbitrary} corruption, we force the user to submit her least preferred item each round to the algorithm over the first $C$ rounds.

\vspace{10pt}
\noindent  \textbf{Baseline Algorithms.} We consider three baseline algorithms for comparison, Doubler \citep{ailon2014reducing}, Sparring \citep{ailon2014reducing}, and Versatile-DB \citep{pmlr-v162-saha22a}. 

\vspace{10pt}
\noindent \textbf{Doubler} is the first approach that transforms a dueling bandit problem into a standard multi-armed bandit (MAB) problem. It operates in epochs of exponentially increasing length: in each epoch, the left arm is sampled from a fixed distribution, and the right arm is selected using a MAB algorithm to minimize regret against the left arm. The feedback received by the MAB algorithm is the number of wins the right arm achieves compared to the left arm. Under linear link assumption, Doubler has been proven to experience regret as the same order as underlying MAB algorithm. For continuous \emph{action} space and general concave utility, we choose Bandit Gradient Descent (BGD, \citep{flaxman2004online}), with regret $O(T^{3/4})$, as the underlying MAB algorithm.

\vspace{10pt}
\noindent \textbf{Sparring} initializes two MAB instances and lets them compete against each other. It is a heuristic improvement over Doubler. Although it does not come with a regret upper bound guarantee, it is reported to enjoy better performance compared to Doubler \citep{ailon2014reducing}. We also choose BGD as the underlying MAB algorithm. 

\vspace{10pt}
\noindent \textbf{Versatile-DB} applies novel reduction approach which converts dueling bandit to MAB. Essentially, it designs simplex over $K$ arms using the idea of follow-the-regularized-leader and updates the simplex using information of whether the arm wins. It has been proved that Versatile-DB is robust to corruption defined as the number of flips of duels and Versatile-DB enjoys regret linear in $C$ \citep{pmlr-v162-saha22a}.

\subsection{Experiments on Synthetic Data}
\subsubsection{DBGD Lower Bound Simulation}\label{sec:lower_bound_simulation}
\textbf{Experiment Setup.} To validate Corollary \ref{theorem:_DBGD_lower_bound}, we construct the following problem instance. Consider the linear utility function $\mu(a) := \theta^{\top}a$. Choose $d = 2, \theta = [\frac{1}{2}, \frac{1}{2}], T=10^5$. Let \emph{action} set $\cA := \{(a_1, a_2): a_1 \geq 0, a_2 \geq 0, \frac{1}{2}a_1 + a_2 - \frac{1}{4} \leq 0\}$. We repeat the experiments for $50$ times, each time with a different seed. 

\vspace{10pt}
\noindent \textbf{Results and Discussion.} Each grey-colored dotted line in Figure \ref{fig:lb} indicate the cumulative regret for each simulation.  The blue line is the average cumulative regret over 50 repeats. The error bar indicates $\pm$ one standard deviation of the regret. The fitted order over the last $1\%$ of the average cumulative regret is 0.76, which is close $0.75$ and supports Corollary \ref{theorem:_DBGD_lower_bound}.

\subsubsection{Regret Upper Bound in Theorem \ref{theorem:regret_lower_bound}}\label{sec:known}

\textbf{Experiment Setup.} To validate regret upper bound in Theorem \ref{theorem:regret_lower_bound}, we consider a strongly concave utility $\mu_{\theta}(a) := \theta^{\top}a - \frac{1}{2}\|a\|^2_2$, a logistic link function $\sigma(x) = \frac{1}{1 + \exp(-x)}$. We choose $d = 5$, and $T = 10^5$. Our \emph{action} space $\cA$ is a $d$-dimensional ball with radius $R = 10$. The preference parameter $\theta$ is randomly sampled from the surface of $\cA$. In our problem setting, the optimal action $a^*$ is $\theta$ and $\mu_{\theta}(a^*) = 50$. We simulate corruption induced by $\rho$-\emph{imperfect} user and conduct experiments for $\rho \in [0.5, 1.0]$. For each value of $\rho$, we repeat the experiments for $5$ times, each under a different seed. We set the learning rate $\eta_{\rho}$ according to Proposition \ref{proposition:matching_upper_bound}.

\begin{wrapfigure}{r}{0pt}
    \centering
    \includegraphics[width=0.4\textwidth]{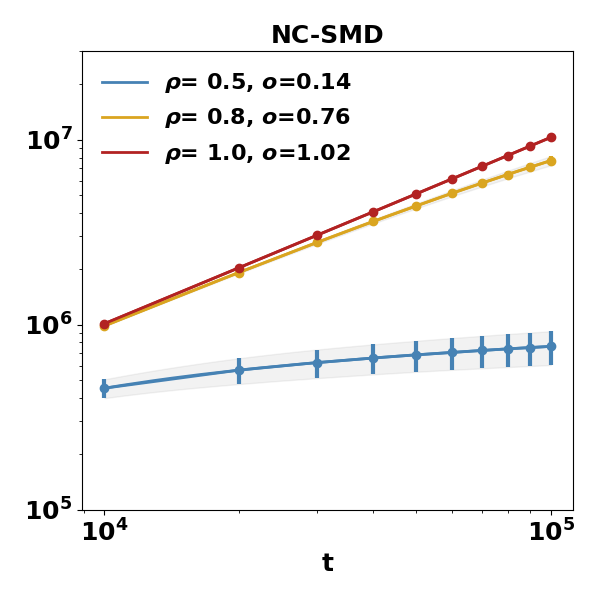}
    \caption{Performance under Known C}
    \label{fig:D1}
\end{wrapfigure}

\vspace{10pt}
\noindent \textbf{Results and Discussion.} Figure \ref{fig:D1} shows that when $\rho$ is known, NC-SMD can tolerate linear $\rho$-\emph{imperfect} user corruption, which confirms theoretical analysis in Proposition \ref{proposition:matching_upper_bound} and implies that lower bound in Theorem \ref{theorem:regret_lower_bound} is tight.

% \begin{figure}[H]
%     \centering
%     \includegraphics[width=0.3\textwidth]{images/known.png}
%     \caption{Performance under Known Corruption}
%     \label{fig:D1}
% \end{figure}

\subsubsection{Robustness under Corruption induced by Imperfect User}\label{sec:robustness}
In Figure \ref{fig:D3}, we simulated the performance of DBGD, NC-SMD, Sparring, Doubler in the same experiment setting as in Section \ref{sec:setup} expect using corruption induced by $\rho$-Imperfect User. We notice that the experiment results also align with theoretical prediction (Theorem \ref{theorem:regret_upper_bound_DBGD} and Proposition \ref{theorem:regret_upper_bound_unknown}), which predicts when $\alpha = 0.25$ for DBGD and $\alpha = 0.5$ for NC-SMD, they can tolerate $O(T^{0.75})$ agnostic corruption. 

\begin{figure}[H]
    \centering
    \includegraphics[width = \textwidth]{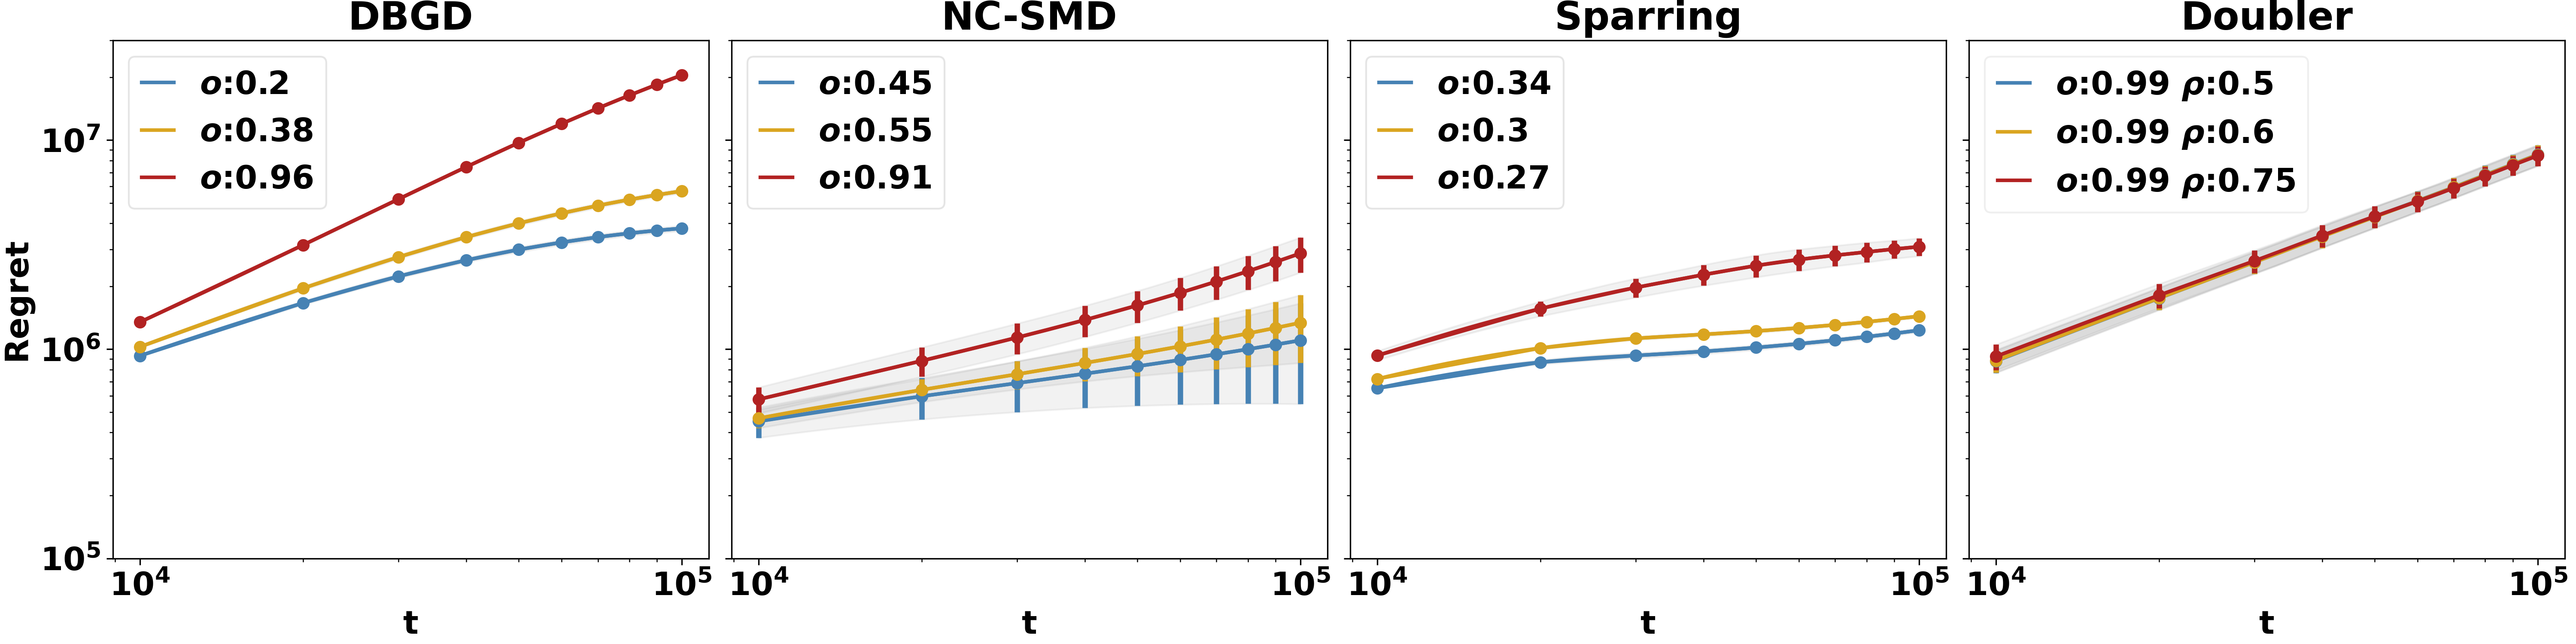}
    \caption{Robustness under Corruption induced by $\rho$-Imperfect User}
    \label{fig:D3}
\end{figure}

\subsubsection{Efficiency-Robustness Tradeoff in Theorem \ref{theorem:regret_upper_bound_DBGD}}\label{sec:tradeoff}
To validate efficiency-robustness trade-off in Theorem \ref{theorem:regret_upper_bound_DBGD} and Proposition \ref{theorem:regret_upper_bound_unknown}, we adopt the same experiment setup as in Section \ref{sec:setup} except different $\alpha$ values. In the first row of Figure \ref{fig:D2}, we consider $\alpha = 0.05$ for DBGD and $\alpha = 0.9$ for NC-SMD. We consider $\rho \in [0.5, 0.95]$. According to the theoretical prediction, both DBGD and NC-SMD can tolerate at most $O(T^{0.95})$ agnostic corruption, which aligns with experiment results. In the second row of Figure \ref{fig:D2}, we consider $\alpha = 0.1$ for DBGD and $\alpha = 0.8$ for NC-SMD. According to the theoretical prediction, both DBGD and NC-SMD can tolerate at most $O(T^{0.9})$ agnostic corruption. From the figure, we can see they have smaller fitted order of regret when $\rho = 0.5$ while at a cost of tolerating smaller magnitude of agnostic corruption (it has linear regret when $\rho = 0.95$), which reveals intrinsic tradeoff between efficiency and robustness. 

\begin{figure}[H]
    \centering
    \includegraphics[width = \textwidth]{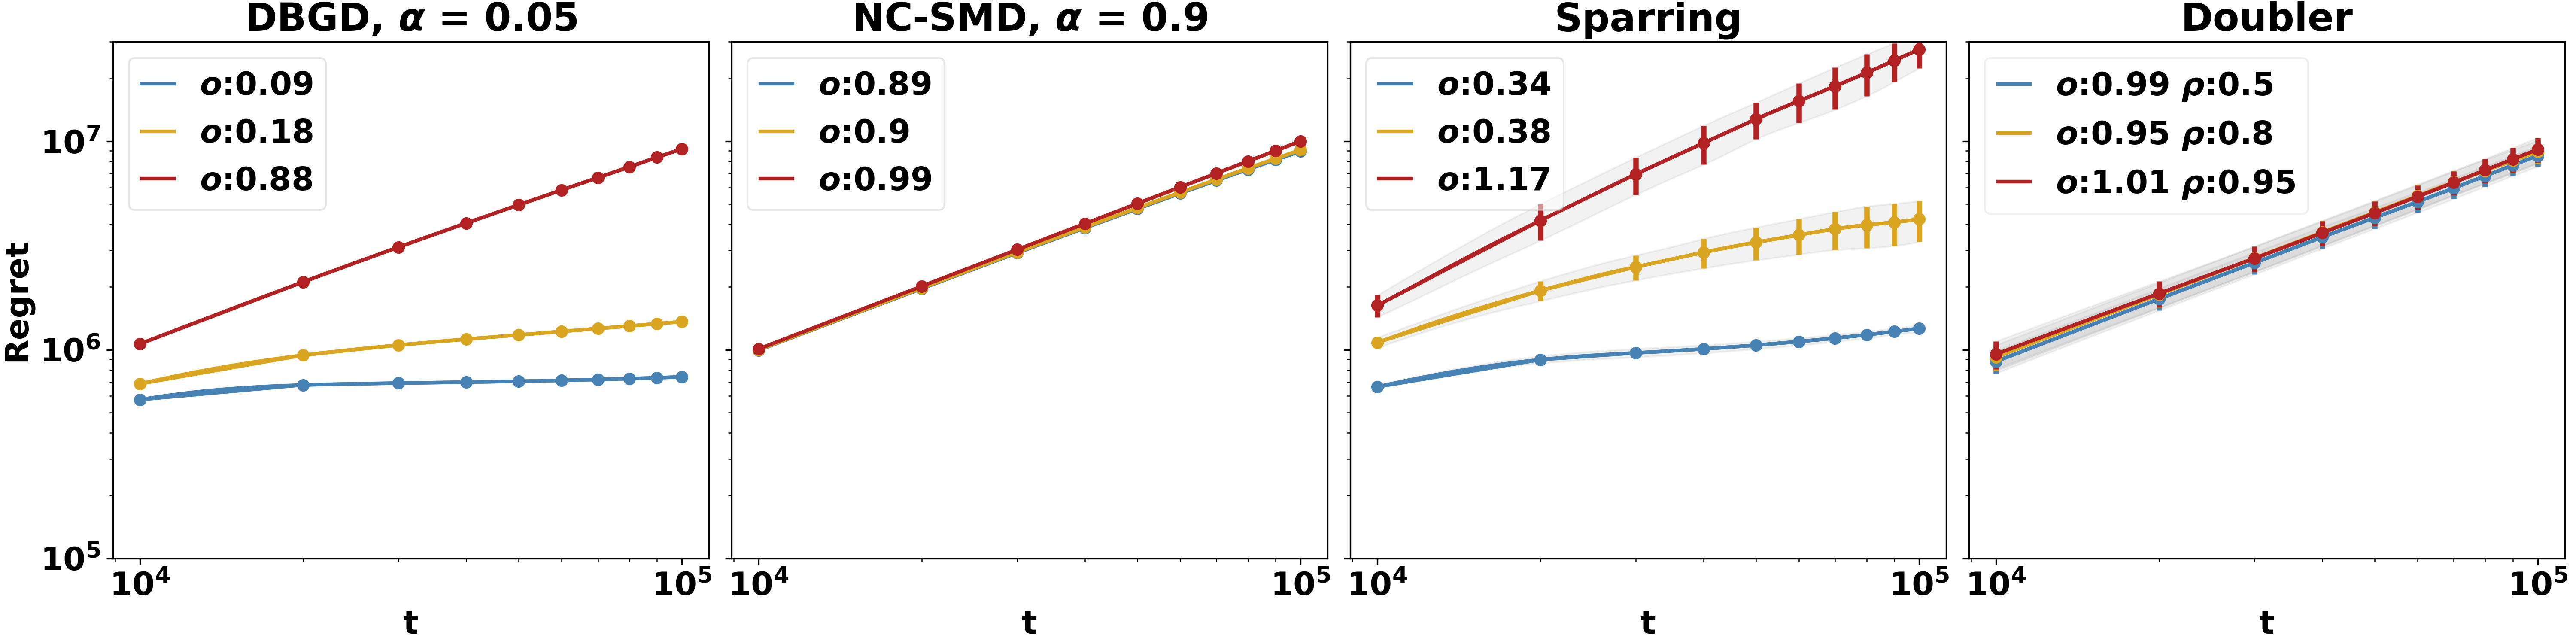}
    \includegraphics[width = \textwidth]{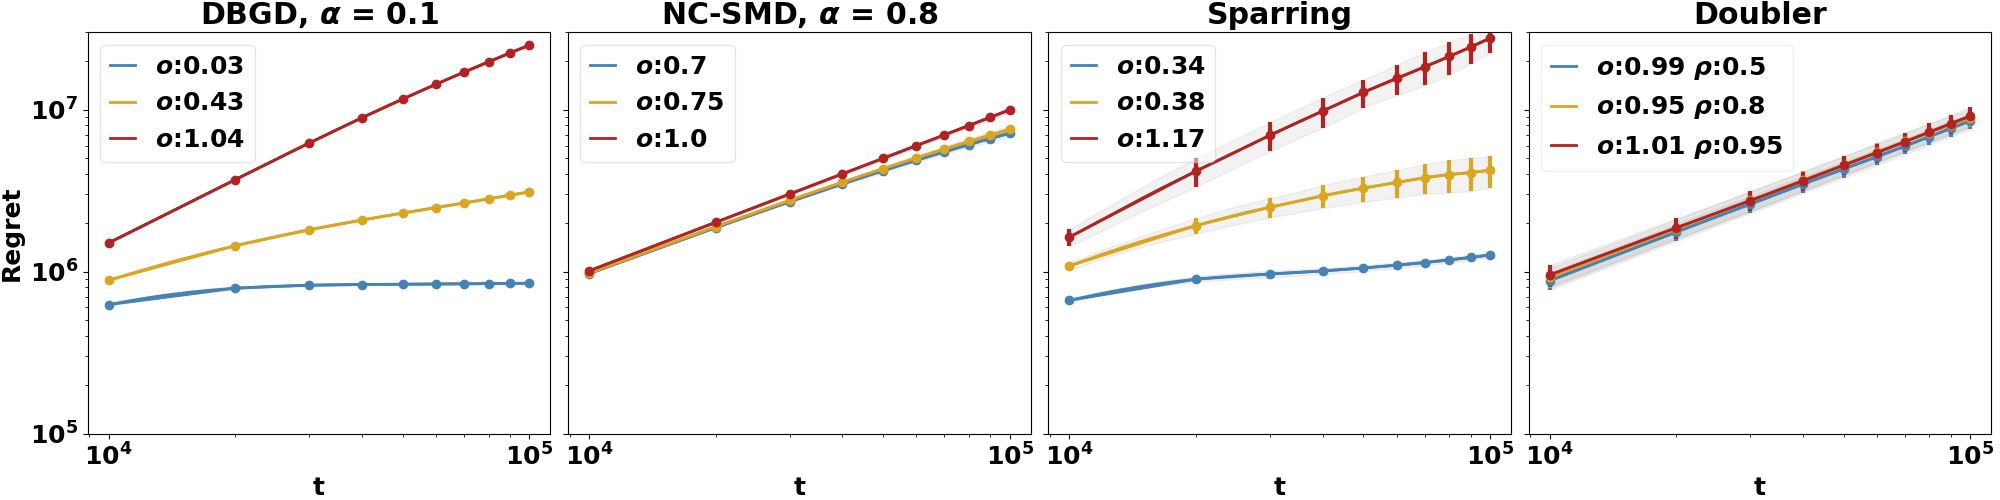}
    \caption{Efficiency-Robustness Tradeoff}
    \label{fig:D2}
\end{figure}

\subsection{Experiments on Spotify Recommendation Data}

\textbf{Evaluation Setup.} We evaluate our approach on Spotify recommendation data \citep{kaggle}. The objective is to recommend songs to incoming users. This dataset includes $17\times 10^4$ songs ($|\cA| = 17\times 10^4$), each is described by 15 distinct features (d = 15). 

\vspace{10pt}
\noindent \textbf{User Profile Identification.} In order to model different types of user, we first use Standard Scaler to standardize the dataset. Then we use Kmeans to conduct clustering \citep{scikit-learn}.

\vspace{10pt}
\noindent \textbf{User Utility.} We use the average of the song embedding within each group as the preference vector. Our aim is to recommend songs to users that have the highest cosine similarity (utility function) with their preference vectors. We rescale the cosine similarity to $[-100, 100]$.

\subsubsection{Performance of Versatile-DB on Spotify Recommendation Data}\label{sec:vdb}
To test the performance of Versatile-DB, we randomly sample $K = 2000$ songs from the Spotify Recommendation Dataset. We identify 2 different user types by clustering the dataset into 2 groups. We use the average of the song embedding within each group as the preference vector and compute the user utility for each recommendation. We consider corruption induced by $\rho$-\emph{imperfect} user for $\rho \in [0.5, 0.75]$. We set $\alpha = 0.25$ for DBGD and run both algorithms for $T = 100$ iterations. This is because Versatile-DB is extremely computationally intensive and running $K = 2000, T=100$ takes around 20 CPU hours. For each user type and for each value of $\rho$, we repeat the experiment over 5 times, each under a different seed. From Figure \ref{fig:D4}, we notice that DBGD outperforms Versatile-DB in all $\rho$, which highlights DBGD's robustness and applicability in real-world data.

\begin{figure}[H]
    \centering
    \includegraphics[width=0.6\textwidth]{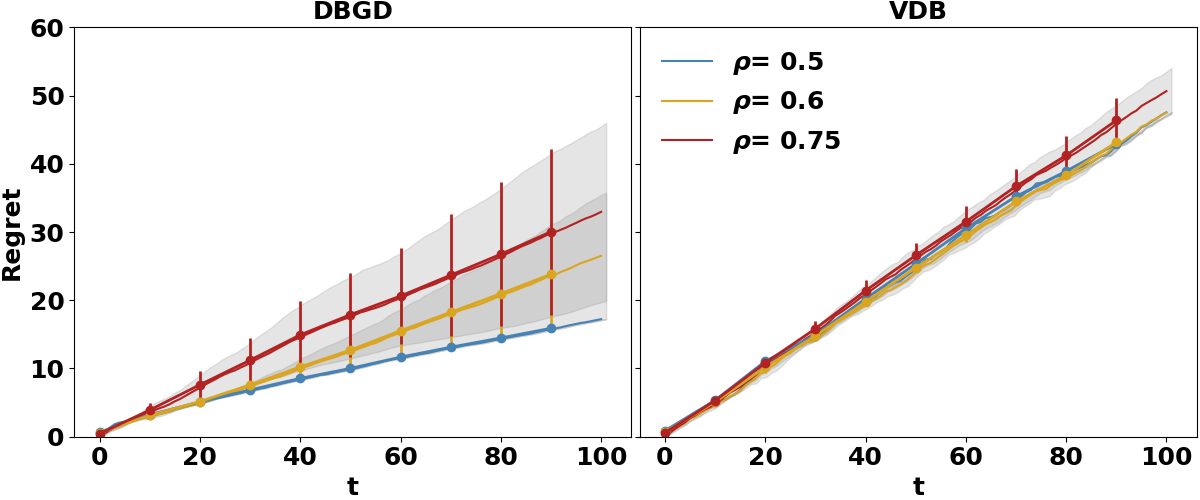}
    \caption{Performance Comparison between DBGD and Versatile-DB}
    \label{fig:D4}
\end{figure}
