# Supplementary material for: Learning from Imperfect Human Feedback: a Tale from Corruption-Robust Dueling
Source: arXiv:2405.11204 source file (2024-10-14)
Supplement: Supplementary file 5 [file appendix-C2.tex]

\subsection{Proof for Matching Regret Upper Bound in Theorem \ref{theorem:regret_lower_bound}}\label{proof:regret_upper_bound}
In this section, we consider the setting when human has strongly concave utility function.  When $\rho$ is known, we optimally adjusts the learning rate of the algorithm, Noisy Comparision-based Stochastic Mirror Descent (NC-SMD), proposed in \cite{kumagai2017regret}, to achieve a balance between optimizing the learning objective \eqref{def:DB_reg} and controlling the gradient bias arising from the \emph{corrupted dueling feedback}. Then we show that it attains the matching regret upper bound of $\Tilde{O}(d\max\{\sqrt{T}, T^{\rho}\})$ under corruption induced by $\rho$-\emph{imperfect} user. 

For the ease of delivering proof, in this section, we work with the cost function $f$, opposite of the utility function $\mu$,  We restate the modelling of inaccuracies from human feedback and the learning objective using $f$ as follows.

\begin{assumption}\textbf{(Corrupted Utility-Based Dueling Bandit).}\label{assumption:decision model_f}
    For a pair of actions $(a, a') \in \cA \times \cA$ and the corruption level $c(a, a')$, there exists function $f: \cA \rightarrow \bR$ and $\sigma: \bR \rightarrow [0, 1]$ such that the probability that $a \succ a'$ happens of receiving \emph{corrupted dueling feedback} can be represented follows
    \begin{equation*}
        \hat \bP(a \succ a')  = \sigma(f(a') - f(a) + c(a,a)).
    \end{equation*}
\end{assumption}
Additionally, we assume that the cost function $f$, the link function $\sigma$, and the action space $\cA$ exhibit the following properties, which align precisely with those assumed in \cite{kumagai2017regret}.
\begin{assumption}\label{assumption:cost function}
    The cost function $f: \cA \rightarrow \bR$ is twice continuously differentiable, $L$-Lipschitz, $\alpha$-strongly convex and $\beta$-smooth with respect to the Euclidean norm.
\end{assumption}
\begin{definition}
   \textbf{ (Strong Convexity).} A function $f: \bR^d \rightarrow \bR$ is $\alpha$-strongly convex over the set $\cA \subset \bR^d$ if for all $x, y \in \cA$ it holds that
    \begin{equation*}
        f(y) \geq f(x) + \nabla f(x)^{\top}(y-x) + \frac{\alpha}{2}\|y - x\|^2_2.
    \end{equation*}
\end{definition}
\begin{definition}
    \textbf{(Smoothness).} A function $f: \bR^d \rightarrow \bR$ is $\beta$-smooth over the set $\cA \subset \bR^d$ if for all $x, y \in \cA$ it holds that
    \begin{equation*}
        f(y) \leq f(x) + \nabla f(x)^{\top}(y-x) + \frac{\beta}{2}\|y - x\|^2_2.
    \end{equation*}
\end{definition}
\begin{assumption}\label{assumption:link function}
    Let $B := \sup_{a, a' \in \cA} f(a') - f(a)$, $f$ is defined in Assumption \ref{assumption:cost function}. The link function $\sigma: \bR \rightarrow [0, 1]$ is three times differentiable and rotational-symmetric. Its first derivative is positive and monotonically non-increasing on $[0, B]$.
\end{assumption}
\begin{assumption}\label{assumption:action space}
    We assume the action space $\cA \in \bR^d$ is convex, compact and has non-empty interior.    
\end{assumption}
\begin{definition}\label{def:self-concordant}
\textbf{(Self-concordance.)}
    A function $\cR: \text{int}(\cA) \rightarrow \bR$ is self-concordant if it satisfies
    \begin{enumerate}
        \item $\cR$ is three times continuously differentiable, convex, and approaches infinity along any sequence of points approaching the boundary of $\text{int}(\cA)$.
        \item For every $h \in \bR^d$ and $x \in \text{int}(\cA)$, $|\nabla^3\cR(x)[h, h, h]| \leq 2\left(h^{\top}\nabla^2\cR(x)h\right)^{\frac{3}{2}}$ holds, where $|\nabla^3\cR(x)[h, h, h]: = \frac{\partial^3\cR}{\partial t_1 \partial t_2 \partial t_3}(x + t_1 h + t_2 h + t_3 h)|_{t_1 = t_2 = t_3 = 0}.$
    \end{enumerate}
In addition to these two conditions, if for every $h \in \bR^d$ and $x \in \text{int}(\cA)$, $|\nabla \cR(x)^{\top}h \leq \nu^{\frac{1}{2}}(h^{\top}\nabla^2\cR(x)h)^{\frac{1}{2}}|$ for a positive real number $\nu$, $\cR$ is $\nu$-self-concordant.
\end{definition}
Through interactions with the user, the learner $\cL$ endeavors to minimize the dueling regret, as defined below.
\begin{equation}\label{def:DB_reg_f}
    \text{Reg}^{\text{DB}}_T = \bE\left(\sum^T_{t=1}\sigma(f(a_t) - f(a^*)) + \sigma(f(a'_t) - f(a^*))-1\right).
\end{equation}
Our minimization objective in \eqref{def:DB_reg_f} aligns with the regret definition in \cite{Yue2009InteractivelyOI}. Under Assumptions \ref{assumption:decision model_f}, \ref{assumption:cost function}, and \ref{assumption:link function}, the regret defined in \eqref{def:DB_reg_f} is equivalent to the regret defined in \cite{kumagai2017regret}. 
Assumption \ref{assumption:cost function} suggests the existence of a unique minimizer $a^*$ for the cost function $f$ due to its strict convexity. Assumptions \ref{assumption:cost function} and \ref{assumption:action space} imply that the diameter $R := \sup_{a, a' \in \mathcal{A}} |a - a'|$ and $B$ are finite. Assumption \ref{assumption:link function} implies the existence of positive constants $l_0$, $L_0$, $B_2$, and $L_2$ such that the first derivative $\sigma'$ of the link function is bounded, satisfying $l_0 \leq \sigma' \leq L_0$ on $[-B, B]$. Furthermore, the second derivative $\sigma^{''}$ is bounded above by $B_2$ and is $L_2$-Lipschitz on $[-B, B]$. Lemma \ref{lemma:s1} establishes the relationship between $\text{Reg}^{\text{FO}}_T$ and $\text{Reg}^{\text{DB}}_T$. 

\begin{lemma}[Lemma 12 in \cite{kumagai2017regret}]\label{lemma:s1}
    \begin{equation}\label{relation}
    \frac{\text{Reg}^{\text{DB}}_T}{L_0} \leq \text{Reg}^{\text{FO}}_T \leq \frac{\text{Reg}^{\text{DB}}_T}{l_0}.
\end{equation}
\end{lemma}

\subsubsection{Noisy Comparison-based Stochastic Mirror Descent}
\begin{algorithm}[H]\label{algo}
\caption{Noisy Comparison-based Stochastic Mirror Descent (NC-SMD)}
\SetKwInput{KwInput}{Input}
\SetKwInOut{KwOutput}{Output}
\KwInput{Learning rate $\eta_\rho$, $\nu$-self-concordant function $\cR$, time horizon $T$, tuning parameters $\lambda$, $\mu$.}
Initialize $a_1 = \arg\min_{a \in A}\cR(a)$\\
\For{$t \in [T]$}
{
Update 
    $\cR_t(a) = \cR(a) + \frac{\lambda\eta_{\rho}}{2}\sum^t_{i = 1}\|a - a_i\|^2 + \mu \|a\|^2$\label{def:self_concordant}
\\
Pick a unit vector $u_t$ uniformly at random\\
Receive the corrupted feedback $\hat{\cF}(a'_t, a_t)$, for $a_t$ and $a'_t = a_t + \nabla^2\cR_t(a_t)^{-1/2}u_t$\\
Compute the corrupted gradient: \label{def:gt_hat}
    $\hat{g}_t = \hat{\cF}(a'_t, a_t)d\nabla^2\cR_t(a_t)^{1/2}u_t$\\
Set $a_{t+1} = \nabla \cR_t^{-1}(\nabla \cR_t(a_t) - \eta_{\rho} \hat{g}_t)$
}
\KwOutput{$a_{T+1}$}
\end{algorithm}
\begin{remark}
Note that $a'_t = a_t + \nabla^2\cR_t(a_t)^{-\frac{1}{2}}x$ for $x \in \bB$ is included in $\cA$ due to the properties of the Dikin ellipsoid.
\end{remark}

Now we begin to prove the matching regret upper bound in Theorem \ref{theorem:regret_lower_bound}.
%%%%%%%%%%%%%%%%%%%%%%%%%%%%%%%%%%%%%%%%%%%%%%%%%%%%%%%%%%%%%%
%Regret upper bound
%%%%%%%%%%%%%%%%%%%%%%%%%%%%%%%%%%%%%%%%%%%%%%%%%%%%%%%%%%%%%%
\begin{proposition}[Full Statement of  Matching Regret Upper Bound in Theorem \ref{theorem:regret_lower_bound}]\label{proposition:matching_upper_bound}
     Let the number of rounds $T$ be fixed and $T > \sqrt{2LL_0 R}$. Consider a corruption induced by $\rho$-\emph{imperfect} user (Def. \ref{def:general-adversary}) with known $\rho$. Under Assumptions \ref{assumption:cost function}, \ref{assumption:link function}, and \ref{assumption:action space}, choose $\lambda \leq l_0 \alpha/2$, $\mu \geq (L^3_0L_2/\lambda)^2$, and set the learning rate $\eta_{\rho} := \frac{\sqrt{\log T}}{dT^{\max\{1/2, \rho\}}}$ for Algorithm \ref{algo}. We have
     we have:
     \begin{equation*}
       \text{Reg}^{\text{DB}}_T \leq O\left(\max\left\{d\sqrt{T\log T}, dT^{\rho}\log T\right\}\right).
     \end{equation*}
\end{proposition}

\begin{proof}
\textbf{(Proof for Proposition \ref{proposition:matching_upper_bound}).}
The formal proof of Proposition \ref{proposition:matching_upper_bound} relies on Lemmas \ref{lemma:bt}, \ref{lemma:error decomposition}, and \ref{lemma: estimation error}. Lemma \ref{lemma:bt} establishes a connection between the gradient estimation corrupted by the bias term $b_t$ and the quantity $\bar P_t(a)$ (defined in Lemma \ref{lemma:bt}), which is the main component we aim to analyze in the regret definition \eqref{def:DB_reg_f}. Lemma \ref{lemma:error decomposition} decomposes the regret into two parts: a regret of decision independent of $b_t$ and an error in observation summarizing the cumulative impact of $b_t$.

The optimization error can be explicitly upper bounded by $T$ and $\eta_{\rho}$ using techniques similar to those employed in \cite{kumagai2017regret}. The upper bound of the estimation error is further established in Lemma \ref{lemma: estimation error}, wherein we utilize the $\alpha$-strong convexity of $f$ to establish a connection between the convergence of the $L_2$-norm of the action $\|a_t - a^*\|_2$ to itself.

\begin{lemma}[Gradient Estimation under Corruption]\label{lemma:bt}
Let $P_t(a)$ represent the likelihood of action $a_t$ being preferred over $a$, where $P_t(a) := \sigma(f(a) - f(a_t))$. Likewise, the corrupted version is defined as $\hat{P}_t(a) = \sigma(f(a) - f(a_t) + c_t(a_t, a'_t))$. The smoothed version of $P_t$ over $\text{int}(\cA)$ is 
$\bar P_t(a): = \bE_{x \in \bB}\left[P_t(a + \nabla^2R_t(a_t)^{-\frac{1}{2}}x)\right]$. $\cR_t(a)$ is defined in Algorithm \ref{algo}. Let $a'_t = a_t + \nabla^2\cR_t(a_t)^{-\frac{1}{2}}u_t$, where $u_t$ is uniformly sampled from $\bS$. Let $b_t := d\left(P_t(a'_t) - \hat P_t(a'_t)\right)\nabla^2\cR_t(a_t)^{\frac{1}{2}}u_t$, we have
    $$\bE\left(\hat g_t | a_t\right) = \nabla \bar P_t(a_t) - \bE \left(b_t | a_t\right).$$
\end{lemma}

\begin{lemma}[Regret Decomposition]\label{lemma:error decomposition}
Define $C_0 := (2\nu + 4L_0\beta + 4B_2 L^2 + LL_0\beta)/\lambda$, and let $a^*_T = \frac{1}{T}a_1 + (1 - \frac{1}{T})a^*$. By Assumption \ref{assumption:link function}, executing Algorithm \ref{algo}, we obtain:
\begin{align*}
    \text{Reg}^{\text{DB}}_T & \leq \underbrace{\frac{C_0}{\eta_{\rho}}\log(T) + 8d^2\eta_{\rho}T + 2LL_0R}_{\textcolor{red}{Regret \hspace{1mm} of\hspace{1mm} Decision}} +  \underbrace{2\bE\left\{\sum^T_{t=1}b^{\top}_t(a_t - a^*_T)\right\}}_{\textcolor{red}{Observation \hspace{1mm} Error}}. 
\end{align*}
\end{lemma}

\begin{lemma}[Estimation Error Upper Bound]\label{lemma: estimation error}
Under Assumption \ref{assumption:cost function}, and \ref{assumption:action space}, we have
    \begin{align*}
    \bE\left\{\sum^T_{t=1}b^{\top}_t(a_t - a^*_T)\right\} 
    & \leq d\sqrt{\lambda \eta_{\rho}}\bE\left\{\sum^T_{t=1}\sqrt{t}m_tn_t\right\} + C_2dC + 2d\sqrt{\lambda \eta_{\rho}T},
    \end{align*}
    where we have $\lambda^*_{\cR}:= \sup_{a \in \cA}\lambda_{\max}\left(\nabla^2\cR(a)\right)$, and $m_t, n_t, C_2$ defined as
    $$m_t := \min\left(2, L_{\sigma}|c_t(a_t, a'_t)|\right), n_t := \min\left(2R, \sqrt{\frac{2}{\alpha}\left(f(a_t) - f(a^*)\right)}\right), C_2 := 2L_{\sigma}R\sqrt{\lambda^*_R + 2\mu}.$$ 
\end{lemma}

Now, we present the proof of Proposition \ref{proposition:matching_upper_bound}. The key technical innovation lies in realizing that the upper bound of $\text{Reg}^{\text{DB}}_T$ contains itself. This implies that we can initially obtain a rough upper bound and then refine it until it becomes tight. The proof follows a mathematical induction argument. For the ease of notation, we reparameterize $C = C_{\kappa}T^{\rho}$. In the following proof, we consider $\rho > 0.5$ to make $T^{\rho} = \max\{\sqrt{T}, T^{\rho}\}$. If $\rho \leq 0.5$, the following proof can be easily modified to make upper bounds involving $T^{\rho}$ as $\sqrt{T}$.

In the first step, we employ a rough upper bound, specifically $\bE\left(n_t\right) \leq 2R$. 
This yields $\text{Reg}^{DB}_{T} \leq O(dT^{\frac{\rho+1}{2}})$. Since $\text{Reg}^{DB}_T$ and $\text{Reg}^{\text{FO}}_T$ share the same order (see Equation \eqref{relation}), it implies that $\sum^T_{t=1}\bE\left(n_t\right)$ must be sublinear as well. Therefore, in the second step, we can use Abel's Summation Equation (Lemma \ref{lemma:abel}) to refine the upper bound of $\bE\left(\sum^T_{t=1}\sqrt{t}m_tn_t\right)$. 

In particular, we rigorously prove the following claim:

\vspace{10pt}

\noindent \textbf{The Induction Claim:}
Given the number of iteration $T$. $T > \sqrt{2LL_0R}$. At k-th step, we have $\text{Reg}^{\text{DB}}_T \leq 144dK\sqrt{\log T} T^{\rho + \frac{\frac{3}{2} - \rho}{2^{k+1}}}$, where $K := \max\left\{C_0, \frac{C_2C_{\kappa}}{\sqrt{\log T}}, L^2_{\sigma}C^2_{\kappa}, 2\sqrt{\lambda}RC_{\kappa}L_{\sigma} \right\}$. 

\vspace{10pt}
\noindent  \textbf{The Base Case:} When $k=1$, let $C_3 = C_2dC + 2d\sqrt{\lambda \eta_{\rho}T}$, we have
\begin{align}
\text{Reg}^{\text{DB}}_T  & \leq \frac{C_0}{\eta_{\rho}}\log(T) + 8d^2\eta_{\rho}T + 2LL_0R + 2C_3 + 2d\sqrt{\lambda \eta_{\rho}}\bE\left(\sum^T_{t=1}\sqrt{t}m_tn_t\right). \label{B1}\\
   & \leq \frac{C_0}{\eta_{\rho}}\log(T) + 8d^2\eta_{\rho}T + 2LL_0R + 2C_3 + 4dR\sqrt{\lambda \eta_{\rho}}\bE\left\{\sum^T_{t=1}\sqrt{t}m_t\right\} \label{B2}\\
    & \leq \frac{C_0}{\eta_{\rho}}\log(T) + 8d^2\eta_{\rho}T + 2LL_0R + 2C_3 + 4dR\sqrt{\lambda \eta_{\rho} T} \left(\sum^T_{t=1}m_t\right)\label{B3}\\
    & \leq  \frac{C_0}{\eta_{\rho}}\log(T) + 8d^2\eta_{\rho}T + 2LL_0R + 2C_3 + 4dL_{\sigma}R\sqrt{\lambda \eta_{\rho}} C_{\kappa}T^{ \rho}\label{B4}.
\end{align}
We get Equation \eqref{B1} according to Lemma \ref{lemma:error decomposition} and \ref{lemma: estimation error}. We get Equation \eqref{B2} because of $\bE\left(n_t\right) \leq 2R$. We get Equation \eqref{B3} by Abel's Summation Equation (see Lemma \ref{lemma:abel}). We get get Equation \eqref{B4} because of corruption budget. Choosing the learning rate $\eta_\rho$ according to Proposition \ref{proposition:matching_upper_bound},  we obtain $\text{Reg}^{\text{DB}}_T \leq 144\sqrt{\log T}K dT^{\frac{\rho + 1}{2}}$. This confirms the validity of the claim when $k=1$.\\

\vspace{10pt}
\noindent \textbf{The Induction Argument:} Let's assume that the claim holds true for a general step $k$. In the following, we will demonstrate that the claim also holds true for step $k+1$. Because of Equation \eqref{relation} and the induction claim, we obtain $\text{Reg}^{\text{FO}}_T \leq \frac{144}{l_0}dK\sqrt{\log T} T^{\rho + \frac{3/2 - \rho}{2^{k+1}}}.$ This suggests that 
\begin{equation*}
    \sum^T_{t=1}\bE\left(f(a_t)-f(a^*)\right) \leq \frac{144}{l_0}dK\sqrt{\log T} T^{\rho + \frac{3/2 - \rho}{2^{k+1}}}.
\end{equation*}
By Jensen's inequality, we have
$$\bE(n_t) = \min\left\{2, \sqrt{\frac{2}{\alpha}}\bE\left(\sqrt{f(a_t) - f(a^*)}\right)\right\} \leq \sqrt{\frac{2}{\alpha}}\sqrt{\bE\left(f(a_t) - f(a^*)\right)}.$$
Therefore we have
\begin{equation*}
    \bE\left(\sum^T_{t=1}\sqrt{t}m_tn_t\right) \leq \sqrt{\frac{2}{\alpha}}\sum^T_{t=1}\sqrt{t}m_t\sqrt{\bE\left(f(a_t) - f(a^*)\right)}.
\end{equation*}
By the definition of monotone adversary, we have $|c_t(a_t, a'_t)|$ is upper bounded by $c_{k}t^{-1 + \rho}$. 
\begin{lemma}\label{lemma:bound}
    Consider $\sum^T_{t=1}n^2_t \leq C'T^{\frac{1}{2} + \alpha}$, with constants $\alpha \geq 0$, $C' > 0$. In addition, $n_t$ is uniformly upper bounded by a constant $K$. Specifically, we have $0 \leq n_t \leq K, \forall t$. $m_t \leq c_kt^{\rho-1}$ with constant $c_k \geq 0$. Then we have $\sum^T_{t=1}\sqrt{t}m_tn_t \leq  5 \sqrt{C'} c_{k}T^{-\frac{1}{4} + \frac{\alpha}{2} + \rho}$. 
\end{lemma}
Therefore, using Lemma \ref{lemma:bound} (details of proof is listed at Appendix \ref{proof:lemma:bound}), we can upper bound $\sqrt{\lambda}\sum^T_{t=1}\sqrt{t}m_tn_t$ by 
\begin{equation*}
    \sqrt{\lambda}\sum^T_{t=1}\sqrt{t}m_tn_t \leq 60L_{\sigma}\sqrt{\frac{2\lambda}{\alpha l_0}}(\log T)^{0.25}C_k\sqrt{dK}T^{\frac{3}{2} \rho + \frac{3/2 - \rho}{2^{k+2}}}
\end{equation*}
Since $\lambda \leq \alpha l_0 /2$, choosing $\eta_{\rho} = \frac{1}{2d}\frac{\sqrt{\log T}}{T^{\rho}}$, we have
\begin{align*}
     \text{Reg}^{\text{DB}}_T & \leq 2d\left(C_0 + \frac{C_2}{\sqrt{\log T}} + 60C_\kappa \sqrt{K}T^{\frac{3/2-\rho}{2^{k+2}}}\right)\sqrt{\log T}T^{\rho} + 12Kd\sqrt{\log T}T^{\rho} \\
     & \leq 144 dK\sqrt{\log T}T^{\rho + \frac{3/2-\rho}{2^{k+2}}}.
\end{align*}
The claim holds true for step $k+1$. Therefore, it implies that the claim holds true for all k. Repeating this process infinitely many times, we obtain $$\text{Reg}^{\text{DB}}_T \leq O\left(d\sqrt{\log T}T^{ \rho}\right),$$
which completes the proof when $\rho \in [0.5, 1]$.
\end{proof}
\subsubsection{Proof for Lemma \ref{lemma:bt}: Gradient Estimation Under Corruption}
\begin{proof}
    \textbf{(Proof for Lemma \ref{lemma:bt}).} If we do not have corruption (i.e. the probability for observing noisy comparative feedback $\cF(a, a') = 1$ is based on true cost difference $f(a') - f(a)$), then the uncorrupted gradient $g_t: = \cF(a'_t, a_t)d\nabla^2\cR_t(a_t)^{1/2}u_t$ should be an unbiased estimate of $\nabla \bar P_t(a_t)$, i.e. $$\bE(g_t | a_t) = \nabla \bar P_t(a_t).$$
    The proof is similar to Lemma 2.1 in \cite{10.5555/1070432.1070486}. Using the Law of total expectation, we have
    \begin{align*}
        \bE(g_t|a_t) & = \bE_{u_t}(\bE( g_t | a_t, u_t))\\
        & = \bE_{u_t}\left(d\bE(P_t(a_t + \nabla^2\cR_t(a_t)^{-\frac{1}{2}}u_t)\nabla^2\cR_t(a_t)^{\frac{1}{2}}u_t|a_t, u_t) \right)\\
        & = d\bE(P_t(a_t + \nabla^2\cR_t(a_t)^{-\frac{1}{2}}u_t)\nabla^2\cR_t(a_t)^{\frac{1}{2}}u_t|a_t)\\
        & = \nabla \bE_{x\in \bB}\left(P_t(a_t + \nabla^2\cR_t(a_t)^{-\frac{1}{2}}x|a_t)\right)\\
        & = \nabla \bar P_t(a_t).
    \end{align*}
We get the second inequality by using the definition of $\cF(a'_t, a_t)$. We use the Stroke's Theorem to get the second last equality. The gradient which we get to perform gradient descent $\hat g_t$  is corrupted. If we let $a'_t = a_t + \nabla^2\cR_t(a_t)^{-\frac{1}{2}}u_t$, we have
\begin{align*}
        \bE(\hat g_t|a_t) & = \bE_{u_t}(\bE(\hat  g_t | a_t, u_t)) \nonumber\\
        & = \bE_{u_t}\left(d\bE(\hat P_t(a'_t)\nabla^2\cR_t(a_t)^{\frac{1}{2}}u_t|a_t, u_t) \right) \nonumber\\
        & = d\bE\left(\hat P_t(a'_t)\nabla^2\cR_t(a_t)^{\frac{1}{2}}u_t|a_t\right) \nonumber\\
        & = d\bE\left(\left[ P_t(a'_t) + \hat P_t(a'_t) - P_t(a'_t)\right]\nabla^2R_t(a_t)^{\frac{1}{2}}u_t|a_t\right)\\
        & = \nabla \bE_{x\in \bB}\left(P_t(a_t + \nabla^2\cR_t(a_t)^{-\frac{1}{2}}x|a_t)\right) + d\bE\left[\left(\hat P_t(a'_t) - P_t(a'_t)\right)\nabla^2\cR_t(a_t)^{\frac{1}{2}}u_t|a_t\right] \nonumber \\
        & = \nabla \bar P_t(a_t) + d\bE\left[\left(\hat P_t(a'_t) - P_t(a'_t)\right)\nabla^2\cR_t(a_t)^{\frac{1}{2}}u_t|a_t\right]\\
        & = \bE(g_t|a_t) + d\bE\left[\left(\hat P_t(a'_t) - P_t(a'_t)\right)\nabla^2\cR_t(a_t)^{\frac{1}{2}}u_t|a_t\right].
\end{align*}
We get the second last equality by using the fact that $g_t$ is unbiased, which we proved earlier. If we defined $b_t$ as 
$$
    b_t := d\left(P_t(a_t + \nabla^2\cR_t(a_t)^{-\frac{1}{2}}u_t) - \hat P_t(a_t + \nabla^2\cR_t(a_t)^{-\frac{1}{2}}u_t)\right)\nabla^2\cR_t(a_t)^{\frac{1}{2}}u_t,
$$
we get 
\begin{equation*}
    \bE(g_t|a_t) = \bE(\hat g_t|a_t) + \bE\left[b_t|a_t\right].
\end{equation*}
\end{proof}
%%%%%%%%%%%%%%%%%%%%%%%%%%%%%%%%%%%%%%%%%%%%%%%%%%%%%%%%%%%%%%%%%%%%%%%%%%%%%%%%%
%%%%%%% Error Decomposition Lemma
%%%%%%%%%%%%%%%%%%%%%%%%%%%%%%%%%%%%%%%%%%%%%%%%%%%%%%%%%%%%%%%%%%%%%%%%%%%%%%%%%

\subsubsection{Proof for Lemma \ref{lemma:error decomposition}: Regret Decomposition}
\begin{proof}
(\textbf{Proof for Lemma \ref{lemma:error decomposition}}). 
% The proof is on Lemma 5 and Lemma 10 in \cite{kumagai2017regret}. 
The cornerstone of the analysis below is to separate the impact of $b_t$ from the total regret. 
\begin{align*}
        & \text{Reg}^{\text{DB}}_T \leq 2\bE\left[\sum^T_{t=1}(P_t(a_t) - P_t(a^*_T)\right] + \frac{LL_0\beta}{\lambda \eta} + 2LL_0R \\
        & \leq 2\left(\bE\left\{\sum^T_{t=1} (\bar P_t(a_t) - \bar P_t(a^*_T)) \right\}
    + \bE\left\{\sum^T_{t=1} (P_t(a_t) - \bar P_t(a_t)) \right\} + \bE\left\{\sum^T_{t=1} (\bar P_t(a^*_T) - P_t(a^*_T)) \right\}\right) \\
    & +  \frac{LL_0\beta}{\lambda \eta} + 2LL_0R\\
    &  \leq 2\bE\left\{\sum^T_{t=1} (\bar P_t(a_t) - \bar P_t(a^*_T))\right\} + \frac{4L_0\beta + 4B_2 L^2 + LL_0\beta}{\lambda \eta_{\rho}}\log T + 2LL_0 R. 
\end{align*}
We get the first inequality by using Lemma \ref{lemma: SA}. We get the last inequality by because 
\begin{equation*}
    \bar P_t(a) - P_t(a) \leq \frac{L_0 \beta + B_2L^2}{2}\| \nabla^2 \cR_t(a_t)^{-\frac{1}{2}}u_t\|^2 \leq \frac{L_0\beta + B_2 L^2}{\lambda \eta_{\rho} t},
\end{equation*}
% $B_2$ is the upper bound for the second derivative of the link function $\sigma$ (see Assumption \ref{assumption:link function}), we have
and
\begin{align*}
     \bE\left\{\sum^T_{t=1} (P_t(a_t) - P_t(a^*_T)) \right\} & \leq \bE\left\{\sum^T_{t=1} (\bar P_t(a_t) - \bar P_t(a^*_T))\right\} + 2\frac{L_0\beta + B_2 L^2}{\lambda \eta_{\rho}}\log T.
\end{align*}
% By the dueling bandit regret definition \eqref{def:DB_reg_f} and Algorithm \ref{algo}, we have

\begin{lemma}[Lemma 5 in \cite{kumagai2017regret}]\label{lemma: SA}
    $$\text{Reg}^{\text{DB}}_T \leq 2\bE\left[\sum^T_{t=1}(P_t(a_t) - P_t(a^*_T)\right] + \frac{LL_0\beta}{\lambda \eta} + 2LL_0R.$$
\end{lemma}

Then it remains to bound $\bE\{\sum^T_{t=1}\bar{P}_t(a_t) - \bar P_t(a^*_T)\}$. And we have the following.
\begin{align*}
    \bE\{\bar{P}_t(a_t) - \bar P_t(a^*_T)\} & \leq \bE\left[\nabla \hat P^{\top}_t(a_t)(a_t - a^*_T) - \frac{l_0 \alpha}{4}\|a_t - a^*_T\|^2\right]\\
    & = \bE\left[g_t^{\top}(a_t - a^*_T) -  \frac{l_0 \alpha}{4}\|a_t - a^*_T\|^2\right]\\ 
    & = \bE\left[(\hat{g}_t + b_t)^{\top}(a_t - a^*_T) -  \frac{l_0 \alpha}{4}\|a_t - a^*_T\|^2\right]\\
    & = \bE\left[\hat{g}_t^{\top}(a_t - a^*_T) -  \frac{l_0 \alpha}{4}\|a_t - a^*_T\|^2\right] + \bE\{b^{\top}_t(a_t - a^*_T)\},
\end{align*}
where the first and second equality is resulted from Lemma \ref{lemma:bt}. Using the definition of $a_{t+1}$ in Algorithm \ref{algo}, we have
$$\nabla \cR_t(a_{t+1}) - \nabla \cR_t(a_t) = \eta_{\rho} \hat{g}_t.$$
Therefore we have
\begin{align*}
    \bE\left[\hat{g}_t^{\top}(a_t - a^*_T) -  \frac{l_0 \alpha}{4}\|a_t - a^*_T\|^2\right]  &
     = \frac{1}{\eta_{\rho}}\bE\left[(\nabla \cR_t(a_{t+1}) - \nabla \cR_t(a_t))^{\top}(a_t - a^*_T) -  \frac{l_0 \alpha \eta_{\rho}}{4}\|a_t - a^*_T\|^2\right]\\
    & = \frac{1}{\eta_{\rho}}\bE\left[D_{\cR_t}(a^*_T, a_t) + D_\cR(a_t, a_{t+1}) - D_{\cR_t}(a^*_T, a_{t+1}) -  \frac{l_0 \alpha \eta_{\rho}}{4}\|a_t - a^*_T\|^2\right].
\end{align*}

$D_{\cR}(a, b)$ is the Bregman divergence associated with $\cR$, defined by
$$D_\cR(a, b) = \cR(a) - \cR(b) - \nabla \cR(b)^\top(a - b).$$
Then we can get Equation \eqref{Es1} by using Lemma \ref{lemma:SB}, \ref{lemma:SC}, \ref{lemma:SD}.
\begin{align}
    \bE\left\{\sum^T_{t=1} (\bar P_t(a_t) - \bar P_t(a^*_T))\right\} \leq \frac{\nu \log(T)}{\eta_{\rho}} + 4 d^2 \eta_{\rho} T + \bE\{\sum^T_{t=1}b_t^{\top}(a_t - a^{*}_T)\}. \label{Es1}
\end{align}

\begin{lemma}[Lemma 10 in \cite{kumagai2017regret}]\label{lemma:SB}
Let $\cR^*_t(a) = \sup_{x \in \bR^d}x^{\top}a - \cR_t(a)$ denote the Frenchel dual of $\cR_t$. Then we have
    \begin{align*}
    & \sum^T_{t=1}\bE\left[\hat{g}_t^{\top}(a_t - a^*_T) -  \frac{l_0 \alpha}{4}\|a_t - a^*_T\|^2\right] \leq \frac{1}{\eta_{\rho}}\left(\cR(a^*_T) - \cR(a_1) + \bE\left[\sum^T_{t=1}D_{\cR^*_t}(\nabla \cR_t(a_t) - \eta_{\rho}\hat{g}_t, \nabla \cR_t(a_t))\right]\right).
\end{align*}
\end{lemma}

\begin{lemma}[Lemma 11 in \cite{kumagai2017regret}]\label{lemma:SC}
When $\eta_{\rho} \leq \frac{1}{2d}$, we have
$$D_{\cR^*_t}(\nabla \cR_t(a_t) - \eta_{\rho}\hat{g}_t, \nabla \cR_t(a_t)) \leq 4d^2\eta^2.$$
\end{lemma}

\begin{lemma}[Lemma 4 in \cite{NIPS2014_c399862d}]\label{lemma:SD}
     $\cR(a^*_T) - \cR(a_1) \leq \nu \log(T).$
\end{lemma}

If we let $C_0 = (2\nu + 4L_0\beta + 4B_2L^2+LL_0\beta)/\lambda$, we have
\begin{align*}
     \text{Reg}^{\text{DB}}_T  & \leq  \frac{2\nu \log(T)}{\eta_{\rho}} + 8 d^2 \eta_{\rho} T + 2\bE\left\{\sum^T_{t=1}b_t^{\top}(a_t - a^{*}_T)\right\} + \frac{4L_0\beta + 4B_2 L^2 + LL_0\beta}{\lambda \eta_{\rho}}\log T + 2LL_0 R\\
     & = \underbrace{\frac{C_0}{\eta_{\rho}}\log(T) + 8d^2\eta_{\rho}T + 2LL_0R}_{\textcolor{red}{Regret \hspace{1mm} of \hspace{1mm} Decision}} +  \underbrace{2\bE\left\{\sum^T_{t=1}b^{\top}_t(a_t - a^*_T)\right\}}_{\textcolor{red}{Observation \hspace{1mm} Error}},
\end{align*}
which completes the proof.
\end{proof}
%%%%%%%%%%%%%%%%%%%%%%%%%%%%%%%%%%%%%%%%%%%%%%%%%%%%%%%%%%%%%%%%%%%%%%%%%%%%%%%%
%%%%%% Upper Bound on Estimation Error
%%%%%%%%%%%%%%%%%%%%%%%%%%%%%%%%%%%%%%%%%%%%%%%%%%%%%%%%%%%%%%%%%%%%%%%%%%%%%%%%
\subsubsection{Proof for Lemma \ref{lemma: estimation error}: Observation Error}
\begin{proof}
    (\textbf{Proof for Lemma \ref{lemma: estimation error}}) In the following, we will analyze the expected cumulative sum of the bias $b_t$ on the total regret, which is $\bE\left\{\sum^T_{t=1}b^{\top}_t(a_t - a^*_T)\right\}$. By Cauchy-Schwarz inequality, $b^{\top}_t(a_t - a^*_T) \leq \|b_t\|_2\|(a_t - a^*_T)\|_2$. We can bound the $\|b_t\|_2$ by the following. 
\begin{align*}
    b^{\top}_tb_t & = d^2\left(P_t(a_t + \nabla^2\cR_t(a_t)^{-\frac{1}{2}}u_t) - \hat P_t(a_t + \nabla^2\cR_t(a_t)^{-\frac{1}{2}}u_t)\right)^2u^{\top}_t\nabla^2\cR_t(a_t)u_t\\
    & \leq \left(P_t(a_t + \nabla^2\cR_t(a_t)^{-\frac{1}{2}}u_t) - \hat P_t(a_t + \nabla^2\cR_t(a_t)^{-\frac{1}{2}}u_t)\right)^2 d^2 \lambda_{\max}(\nabla^2\cR_t(a_t)).
\end{align*}
We get the first equality by Lemma $\ref{lemma:bt}$. We get the inequality by using the fact $\|u_t\|_2 = 1$. If we let $a'_t = a_t + \nabla^2\cR_t(a_t)^{-\frac{1}{2}}u_t$, then we have
\begin{align*}
    |P_t(a'_t) - \hat P_t(a'_t)| & = |\sigma(f(a_t) - f(a'_t)) - \sigma(f(a_t) - f(a'_t) + c_t(a_t, a'_t))|\\
    & \leq \min \left(2, L_{\sigma}|c_t(a_t, a'_t)|\right).
\end{align*}
We get the first equality by using the definition of $P_t(a_t)$ and $\hat P_t(a_t)$. We get the first inequality by using the Lipschitz property of $\sigma$ (see Assumption \ref{assumption:link function})
Therefore, we have $$\|b_t\|_2 \leq d\sqrt{\lambda_{\max}(\nabla^2\cR_t(a_t))}\min\left\{2, L_{\sigma}|c_t(a_t, a'_t)|\right\}.$$ 
If we use $\lambda^*_R:= \sup_{a \in \cA}\lambda_{\max}\left(\nabla^2\cR(a)\right)$, then we have
\begin{align*}
    \lambda_{\max}(\nabla^2 \cR_t(a_t)) & = \lambda_{\max}(\nabla^2 \cR(a_t)) + \lambda \eta_{\rho}t + 2\mu
    \leq  \lambda^*_R + 2\mu + \lambda \eta_{\rho}t.
\end{align*}

Therefore we have
\begin{align}
    & \bE\left\{\sum^T_{t=1}b^{\top}_t(a_t - a^*_T)\right\}  \leq \bE\left\{\sum^T_{t=1}\|b_t\|_2\|a_t - a^*_T\|_2\right\} \nonumber \\
    & \leq \bE\left\{\sum^T_{t=1}(d\sqrt{\lambda_{\max}(\nabla^2\cR_t(a_t))} \min \left(2, L_{\sigma}|c_t(a_t, a'_t)|\right))\|a_t - a^*_T\|_2\right\} \nonumber\\
    & \leq \bE\left\{\sum^T_{t=1}(d\sqrt{\lambda^*_R + 2\mu + \lambda \eta_{\rho}t} \min \left(2, L_{\sigma}|c_t(a_t, a'_t)|\right))\|a_t - a^*_T\|_2\right\} \nonumber\\
    & \leq \bE\left\{\sum^T_{t=1}(d\sqrt{\lambda^*_R + 2\mu}  \min \left(2, L_{\sigma}|c_t(a_t, a'_t)|\right)\|a_t - a^*_T\|_2\right\} + \bE\left\{\sum^T_{t=1}(d\sqrt{\lambda \eta_{\rho}t} \min \left(2, L_{\sigma}|c_t(a_t, a'_t)|\right)\|a_t - a^*_T\|_2\right\} \nonumber\\
    & \leq 2RdL_{\sigma}\sqrt{\lambda^*_R + 2\mu}C + d\sqrt{\lambda \eta_{\rho}}\bE\left\{\sum^T_{t=1}\sqrt{t} \min \left(2, L_{\sigma}|c_t(a_t, a'_t)|\right)\|a_t - a^*_T\|_2\right\} \label{SE1}\\
    & \leq 2RdL_{\sigma}\sqrt{\lambda^*_R + 2\mu}C + 2d\sqrt{\lambda\eta_{\rho}T} + d\sqrt{\lambda \eta_{\rho}}\bE\left\{\sum^T_{t=1}\sqrt{t} \min \left(2, L_{\sigma}|c_t(a_t, a'_t)|\right)\|a_t - a^*\|_2\right\} \label{SE2}\\
    & \leq 2RdL_{\sigma}\sqrt{\lambda^*_R + 2\mu}C + 2d\sqrt{\lambda\eta_{\rho}T} + d\sqrt{\lambda \eta_{\rho}}\bE\left\{\sum^T_{t=1}\sqrt{t} \min \left(2, L_{\sigma}|c_t(a_t, a'_t)|\right)\min\left(2R, \sqrt{\frac{2}{\alpha} \left(f(a_t) - f(a^*)\right)}\right)\right\}\nonumber.
\end{align}
We get Equation \eqref{SE1} by using the fact that $\|a_t - a^*_T\|_2 \leq 2R$, $\sum^T_{t=1}|c_t(a_t, a'_t)| \leq C$. We get Equation \eqref{SE2} the definition of $a^*_T$, and the fact $\sqrt{a + b} \leq \sqrt{a} + \sqrt{b}$. Using the $\alpha$-strong convexity of $f$ (see Assumption \ref{assumption:cost function}), we have $ \|a_t - a_*\|_2 \leq \min\left(2R, \sqrt{\frac{2}{\alpha} \left(f(a_t) - f(a^*)\right)}\right)$ we get the last inequality, which completes the proof.
\end{proof}
\subsubsection{Proof for Lemma \ref{lemma:bound}}\label{proof:lemma:bound}

\begin{proof}
\textbf{(Proof for Lemma \ref{lemma:bound}).}
Using Abel's Summation Equation (Lemma \ref{lemma:abel}), we have
\begin{equation*}
    \sum^T_{t=1}\sqrt{t}m_tn_t \leq \sqrt{T}\left(\sum^T_{t=1}m_tn_t\right)
\end{equation*}
Since we have $\sum^T_{t=1}n^2_t \leq C'T^{\frac{1}{2} + \alpha}$ and $0 \leq n_t \leq K, \forall t$, we have $\sum^T_{t=1}n_t \leq \sqrt{C'} T^{\frac{3}{4} + \frac{\alpha}{2}}, \forall t$.  Moreover, for $t \geq 1$, $t^{-1 + \rho} - (t+1)^{-1 + \rho} \leq t^{\rho - \frac{1}{2}}$ holds for all $t \geq 1$. This is because
\begin{equation*}
    f(t) = t^{-1 + \rho}\left((1 +\frac{1}{t})^{-1 + \rho} + \frac{1}{t} -  1\right).
\end{equation*}
is decreasing over $t \geq 1$ and $\lim_{t \rightarrow \infty} f(t) = 0$. Consequently, applying Abel's Summation Equation again, we have
\begin{align*}
    \sum^T_{t=1}m_tn_t &=  \left(\sum^T_{t=1}n_t\right)m_T + \sum^{T-1}_{t=1}\left(\sum^t_{i=1}n_i\right)(m_t - m_{t+1})\\
    & \leq \sqrt{C'}c_{k}T^{\frac{3}{4}+\frac{\alpha}{2}}T^{-1 + \rho} + \sqrt{C'}c_{k} \sum^{T-1}_{t=1}\left(\sum^t_{i=1}n_i\right) \left(t^{-1+ \rho} - (t+1)^{-1 + \rho}\right)\\
    & \leq \sqrt{C'}c_{k}T^{\frac{3}{4}+\frac{\alpha}{2}}T^{-1 + \rho} + \sqrt{C'}c_{k} \sum^{T-1}_{t=1}\left(\sum^t_{i=1}n_i\right)t^{-\frac{1}{2} + \rho}\\
    & \leq \sqrt{C'}c_{k}T^{\frac{3}{4}+\frac{\alpha}{2}}T^{-1 + \rho} + \sqrt{C'}c_{k} \sum^{T-1}_{t=1}t^{\frac{3}{4} + \frac{\alpha}{2}}t^{-\frac{1}{2} + \rho}\\
    & \leq 5 \sqrt{C'} c_{k}T^{-\frac{1}{4} + \frac{\alpha}{2} + \rho}.
\end{align*}
Since $0 \leq n_t \leq K$, $\sum^t_{i=1}n_i$ is increasing and the increasing rate is upper bound by $t$. Together with the constraint $\sum^T_{t=1}n_t \leq \sqrt{C'}T^{\frac{3}{4} + \frac{\alpha}{2}}$, $\sum^{T-1}_{t=1}\left(\sum^t_{i=1}n_i\right)t^{-\frac{1}{2} + \rho}$ is optimized when $\sum^t_{i=1}n_i$ increasing in the speed of $\sqrt{C'}t^{\frac{3}{4} + \frac{\alpha}{2}}$. Because of this, the second last inequality holds. 
\begin{lemma}\label{lemma:abel}
    \textbf{(Abel's Summation Equation \citep{williams1963class}).} For any numbers $a_k$, $b_k$, we have
    \begin{equation*}
        \sum^n_{k=1}a_kb_k = \left(\sum^n_{k=1}b_k\right)a_n + \sum^{n-1}_{k=1}\left(\sum^{k}_{i=1}b_i\right)(a_k - a_{k+1}).
    \end{equation*}
\end{lemma}
\end{proof}

\subsection{Proof for Proposition \ref{theorem:regret_upper_bound_unknown}: Efficiency-Robustness Tradeoff in NC-SMD}\label{proof:theorem:regret_upper_bound_unknown}
\begin{retheorem}[Full Statement of Proposition \ref{theorem:regret_upper_bound_unknown}] Let the number of rounds $T$ be fixed and $T > \sqrt{2LL_0 R}$. Under Assumptions \ref{assumption:cost function}, \ref{assumption:link function}, and \ref{assumption:action space}, by choosing $\lambda \leq l_0 \alpha/2$, $\mu \geq (L^3_0L_2/\lambda)^2$, and setting the learning parameter $\eta_{\rho} = \frac{\sqrt{\log T}}{2d}T^{-\alpha}, \alpha \in [0.5, 1]$, regret occurred by Algorithm \ref{algo} satisfies 
 \begin{equation*}
        \text{Reg}_T \leq \Tilde{O}\left(dT^{\alpha} + \sqrt{d}T^{\frac{1}{2}(1-\alpha)}C + dC\right)
 \end{equation*}
for any corruption with budget $C$.
\end{retheorem}
\begin{proof}
    \textbf{(Proof for Proposition \ref{theorem:regret_upper_bound_unknown}).}
From Lemma \ref{lemma: estimation error}, we know
\begin{align*}
     \bE\left\{\sum^T_{t=1}b^\top_t(a_t - a^*_T)\right\} & \leq 2RdL_{\sigma}\sqrt{\lambda^*_R + 2\mu}C + d\sqrt{\lambda \eta_{\rho}}\bE\left\{\sum^T_{t=1}\sqrt{t} \min \left(2, L_{\sigma}|c_t(a_t, a'_t)|\right)\|a_t - a^*_T\|_2\right\}\\
     & \leq 2RdL_{\sigma}\sqrt{\lambda^*_R + 2\mu}C + 2Rd\sqrt{\lambda \eta_{\rho}}L_{\sigma}\sum^T_{t=1}\sqrt{t}|c_t(a_t, a'_t)|\\
     & \leq 2RdL_{\sigma}\sqrt{\lambda^*_R + 2\mu}C + 2Rd\sqrt{\lambda \eta_{\rho}T}L_{\sigma}C.
\end{align*}
We get the second inequality by using the fact that the diameter of the action space of $R$. We get the last inequality by using Abel Summation Equation (see Lemma \ref{lemma:abel}). Therefore, by Lemma \ref{lemma:error decomposition}, we have
\begin{align*}
    \text{Reg}_T \leq \frac{C_0}{\eta_{\rho}}\log(T) + 8d^2\eta_{\rho}T + 2LL_0R + 4RdL_{\sigma}\sqrt{\lambda^*_R + 2\mu}C+ 4Rd\sqrt{\lambda \eta_{\rho}T}L_{\sigma}C.
\end{align*}
Choosing $\eta_{\rho} = \frac{\sqrt{\log T}}{2d}T^{-\alpha}, \alpha \in [0.5, 1]$, we have
\begin{align*}
    \text{Reg}_T  & \leq 2dC_0\sqrt{\log T}T^{\alpha} + 4d\sqrt{\log T}T^{1-\alpha} + 4RdL_{\sigma}\sqrt{\lambda^*_R + 2\mu}C + 4R\sqrt{d}L_{\sigma}(\log T)^{0.25}T^{\frac{1}{2}(1-\alpha)}C + 2LL_0R\\
    & \leq O\left(d\sqrt{\log T}T^{\alpha} + \sqrt{d}(\log T)^{\frac{1}{4}} T^{\frac{1}{2}(1 - \alpha)}C + dC\right),
\end{align*}
which completes the proof.
\end{proof}
